# Supplementary material for: BridgeIV: Bridging Customized Image and Video Generation through Test-Time Autoregressive Identity Propagation
Source: arXiv:2505.06985 source file (2025-05-11)
Supplement: Supplementary file 2 [file supplement_0.tex]

\section{Supplemental Experiments}
\subsection{Implementation Details}

\subsection{Results}

\noindent \textbf{Qualitative Results.}
\begin{figure*}[ht!]
\centering
\includegraphics[width=1\textwidth]{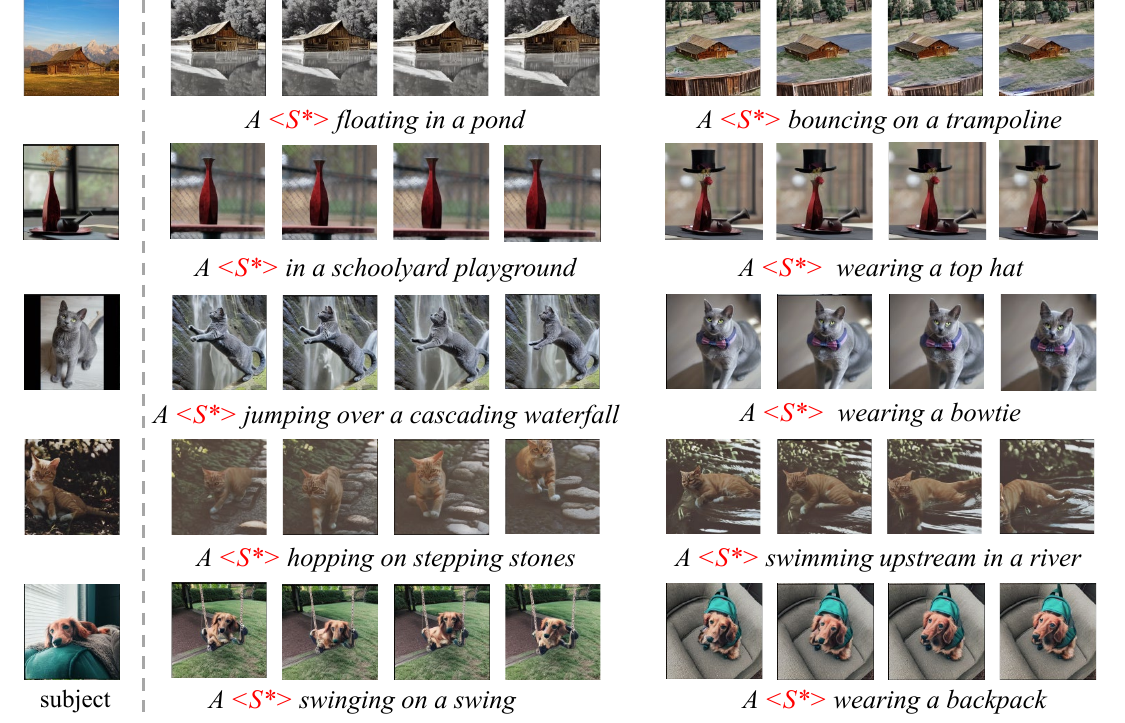} 
\caption{The visualization of qualitative results. }
% \Description{We recommend the reader to zoom in to read the details.}
\label{fig:qualitative results}
\end{figure*}

\noindent \textbf{Failure Cases.}
\begin{figure}[ht!]
\centering
\includegraphics[width=0.5\textwidth]{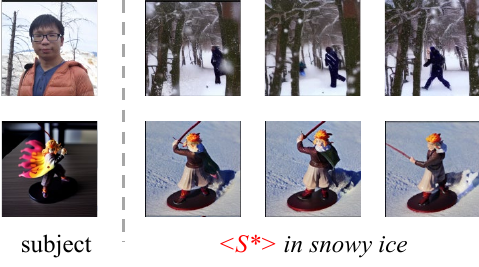} 
\caption{The visualization of two failure cases.}
% \Description{We recommend the reader to zoom in to read the details.}
\label{fig:failure cases}
\end{figure}
